# Supplementary material for: C-RAG: Certified Generation Risks for Retrieval-Augmented Language Models
Source: arXiv:2402.03181 source file (2024-07-30)
Supplement: Supplementary file 1 [file legacy.tex]

The contrastive loss (triplet loss) with encoder $f_r(\cdot): \gX \mapsto \sR^d$ can be formulated as:

Loss 1:
\begin{equation}
    \gL_{\text{contr}}(x,x^+,x^-) = \max \left\{ \|f_r(x) - f_r(x^+)\|_2 - \| f_r(x) - f_r(x^-) \|_2 + t , 0 \right\},
\end{equation}
where $t>0$ is a margin constant in the triplet loss.

Loss 2:
\begin{equation}
    \gL_{\text{contr}}(x,x^+,x^-) = - \log \dfrac{\exp\left\{\text{sim}(x,x^+)\right\}}{\exp\left\{\text{sim}(x,x^+)\right\} + \exp\left\{\text{sim}(x,x^-)\right\} }
\end{equation}

Since the encoder of the retriever $f_r(\cdot)$ is trained with the contrastive loss, we suppose that the contrastive loss is bounded with a constant $L_\tau~(L_\tau < t)$.
Let $\gD_{\text{ext}}^+(x)$, $\gD_{\text{ext}}^-(x)$ be the positive and negative samples of $x$ in the external knowledge base.
Positive examples and negative examples are defined as examples with the same/different groundtruth output.
Let $\gD$ be the data distribution where training, calibration, and test samples are drawn from.
Then we have:

Loss 1:
\begin{equation}
    \mathbb{E}_{x\sim \gD, x^+ \sim \gD^+_{\text{ext}}(x), x^- \sim \gD^-_{\text{ext}}(x)}\left[ \gL_{\text{contr}}(x,x^+,x^-) \right] \le L_\tau,
\end{equation}
which implies the following:
\begin{equation}
    \mathbb{E}_{x\sim \gD, x^+ \sim \gD^+_{\text{ext}}(x), x^- \sim \gD^-_{\text{ext}}(x)}\left[ \|f_r(x) - f_r(x^+)\|_2 - \| f_r(x) - f_r(x^-) \|_2 \right] \le L_\tau - t.
\end{equation}

Loss 2:
\begin{equation}
    \mathbb{E}_{x\sim \gD, x^+ \sim \gD^+_{\text{ext}}(x), x^- \sim \gD^-_{\text{ext}}(x)}\left[ \gL_{\text{contr}}(x,x^+,x^-) \right] \le L_\tau,
\end{equation}
which implies the following:
\begin{equation}
    \mathbb{E}_{x\sim \gD, x^+ \sim \gD^+_{\text{ext}}(x), x^- \sim \gD^-_{\text{ext}}(x)}\left[ \text{sim}(x,x^+) - \text{sim}(x,x^-) \right] \ge \ln \dfrac{\exp\left\{ -L_\tau \right\}}{1 - \exp\left\{ -L_\tau \right\}}.
\end{equation}

Loss 1:
Suppose that the norm of embedding $\|f_r(x)\|_2$ for any $x \in \gX$ is bounded by a positive constant $B$: $\sup_{x\in \gX} \|f_r(x)\|_2 \le B$.
Then from Chebyshev's inequality, we have:
\begin{equation}
    \sP_{x\sim \gD, x^+ \sim \gD^+_{\text{ext}}(x), x^- \sim \gD^-_{\text{ext}}(x)}\left[ \|f_r(x) - f_r(x^+)\|_2 > \| f_r(x) - f_r(x^-) \|_2 \right] \le \dfrac{\mathbb{V}\left[\|f_r(x) - f_r(x^+)\|_2 - \| f_r(x) - f_r(x^-) \|_2\right]}{(t - L_\tau)^2}:=\delta
\end{equation}

Loss 2:
Suppose that we have $0 \le \text{sim}(\cdot,\cdot) \le 1$.
Then from Chebyshev's inequality, we have:
\begin{align}
    \sP_{x\sim \gD, x^+ \sim \gD^+_{\text{ext}}(x), x^- \sim \gD^-_{\text{ext}}(x)}\left[ \text{sim}(x,x^+) < \text{sim}(x,x^-) \right] &\le \dfrac{\mathbb{V}\left[\text{sim}(x,x^+) - \text{sim}(x,x^-)\right]}{\left(\ln \dfrac{\exp\left\{ -L_\tau \right\}}{1 - \exp\left\{ -L_\tau \right\}} \right)^2} \\
    &\le \dfrac{ \left( \sqrt{\mathbb{V}\left[\text{sim}(x,x^+)\right]} + \sqrt{\mathbb{V}\left[\text{sim}(x,x^-)\right]} \right)^2 }{\left(\ln \dfrac{\exp\left\{ -L_\tau \right\}}{1 - \exp\left\{ -L_\tau \right\}} \right)^2} \\
    &\le \left(\ln \dfrac{\exp\left\{ -L_\tau \right\}}{1 - \exp\left\{ -L_\tau \right\}} \right)^{-2} := \delta
\end{align}

We first consider one example retrieved with the highest similarity to $Z_q$: $Z_r$. Without loss of generality, we let the groundtruth output of example $Z_q$ be $c$. Let $\gD_{\text{ext}}^{(c)}$ be the set of examples with groundtruth output $c$ in the external knowledge base. 
Let $r_c^{\text{(cal)}}$ and $r_c^{\text{(ext)}}$ be the $c$-th event probability of the categorical distribution of calibrations samples and the samples from the external knowledge base.
The concentration bound of the categorical distribution is formulated as follows \cite{agrawal2017optimistic}:
\begin{align}
    % \sP\left[ \|\hat{\vr}_{\text{cal}} - \vr_{\text{cal}} \|_1 \ge \dfrac{\sqrt{2\ln{(1/\delta_{\text{cal}})}}}{N_{\text{cal}}} \right] \le \delta_{\text{cal}}, \\
    \sP\left[ \|\hat{\vr}_{\text{ext}} - \vr_{\text{ext}} \|_1 \ge \dfrac{\sqrt{2\ln{(1/\delta_{\text{ext}})}}}{N_{\text{ext}}} \right] \le \delta_{\text{ext}}.
\end{align}

Then $\forall \delta_{\text{ext}}$ with probability $1-\delta_{\text{ext}}$, we have:

loss 1:
\begin{align}
    \sP\left[ Z_r \notin  \gD_{\text{ext}}^{(c)}\right] &= \sP_{z_q \sim \gD_{\text{cal}}}\left[ \|f_r(z_q) - f_r(Z_r)\|_2 < \min_{z \in \gD_{\text{ext}}^{(c)}} \|f_r(z_q) - f_r(z)\|_2 \right] \\
    % &\le \sP_{Z_q \sim \gD_{\text{cal}}, z^+ \sim \gD^+_{\text{ext}}(Z_q)}\left[ \|f_r(z_q) - f_r(Z_r)\|_2 <  \|f_r(Z_q) - f_r(z^+)\|_2 \right] \\
    &\le \sP_{z_q \sim \gD_{\text{cal}}}\left[ \min_{z^- \in \gD^-_{\text{ext}}(z_q)}  \|f_r(z_q) - f_r(z^-)\|_2 <  \min_{z^+ \in \gD^+_{\text{ext}}(z_q)} \|f_r(z_q) - f_r(z^+)\|_2 \right] \\
    &\le \sum_{c=1}^C r_c^{\text{cal}} \left(1 - r_c^{\text{(ext)}} + \dfrac{\sqrt{2\ln{(1/\delta_{\text{ext}})}}}{N_{\text{ext}}} \right) N_{\text{ext}} \delta^{N_{\text{ext}} \left(r_c^{\text{(ext)}} - \dfrac{\sqrt{2\ln{(1/\delta_{\text{ext}})}}}{N_{\text{ext}}} \right)}
\end{align}

loss 2:
\begin{align}
    \sP\left[ Z_r \notin  \gD_{\text{ext}}^{(c)}\right] &= \sP_{z_q \sim \gD_{\text{cal}}}\left[ \text{sim}(z_q, Z_r) \ge \max_{z \in \gD_{\text{ext}}^{(c)}} \text{sim} (z_q, z) \right] \\
    &\le \sP_{z_q \sim \gD_{\text{cal}}}\left[ \max_{z^- \in \gD^-_{\text{ext}}(z_q)}  \text{sim}(z_q, z^-) \ge  \max_{z^+ \in \gD^+_{\text{ext}}(z_q)} \text{sim}(z_q, z^+) \right] \\
    &\le \sum_{c=1}^C r_c^{\text{cal}} \left(1 - r_c^{\text{(ext)}} + \dfrac{\sqrt{2\ln{(1/\delta_{\text{ext}})}}}{N_{\text{ext}}} \right) N_{\text{ext}} \delta^{N_{\text{ext}} \left(r_c^{\text{(ext)}} - \dfrac{\sqrt{2\ln{(1/\delta_{\text{ext}})}}}{N_{\text{ext}}} \right)}
\end{align}

Let $\delta_c=\delta_{\text{ext}}$.
Then we have:
\begin{equation}
    \sP\left[ Z_r \notin  \gD_{\text{ext}}^{(c)}\right] \le \min_{\delta_c} (1-\delta_c) \left(\sum_{c=1}^C r_c^{\text{cal}}\left(N_{\text{ext}} - N_{\text{ext}} r_c^{\text{(ext)}} + {\sqrt{2\ln{(1/\delta_c)}}} \right)  \delta^{ N_{\text{ext}}r_c^{\text{(ext)}} - {\sqrt{2\ln{(1/\delta_c)}}} }  \right) + \delta_c
\end{equation}

Let $N_{\text{pos}}$ be the number of positive examples in the context.
We assume that the in-context examples are retrieved identically and independently, then we have:
\begin{equation}
    \mathbb{E}\left[ N_{\text{pos}} \right] \ge \max_{\delta_c} N_{\text{cont}} \left(1-\delta_c\right)\left(1- \sum_{c=1}^C r_c^{\text{cal}} \left(N_{\text{ext}} - N_{\text{ext}} r_c^{\text{(ext)}} + {\sqrt{2\ln{(1/\delta_c)}}} \right)  \delta^{ N_{\text{ext}}r_c^{\text{(ext)}} - {\sqrt{2\ln{(1/\delta_c)}}} }  \right)
\end{equation}

Assume that $\max_{c \neq g} O'(\vq_N)c - O'(\vq_N)_g$ follows a Gaussian mixture $k_1 \gN(\mu_1,\sigma_1^2)+k_2 \gN(\mu_2,\sigma_2^2)$ $\mu_1 < 0 < \mu_2$.
Then with probability $1 - \dfrac{\mathbb{V}[N_{\text{pos}}]}{(\underline{N}_{\text{pos}}-n)^2}$, we have:
\begin{align}
    \mathbb{E}\left[ R - R_{\text{rag}} \right] &\ge \sum_{i=0}^1 k_i \left(\text{CDF}_i\left( n (d^++d^-) - N_{\text{cont}} d^-)(t^+-t^-) \right) - \text{CDF}_i(0) \right) := \tau(n)
\end{align}

Gaussian may be a strong one, so we can consider a relaxed assumption to quantify the imperfectiveness of the case without RAG:
\begin{equation}
    \text{CDF}(v) = \sP\left[ \max_{c \neq g} O'(\vq_N)c - O'(\vq_N)_g < v \right],
\end{equation}
with which we can define:
\begin{equation}
    \tau(n) = \text{CDF}\left( n (d^++d^-) - N_{\text{cont}} d^-)(t^+-t^-) \right) - \text{CDF}(0)
\end{equation}
and we have the following (Improved version):
\begin{align}
    & \mathbb{E}\left[ R - R_{\text{rag}} \right] \\ 
    =& \mathbb{E} \left[ \text{CDF}\left( N_{\text{pos}} (d^++d^-) - N_{\text{cont}} d^-)(t^+-t^-) \right) \right] - \text{CDF}(0) \\
    \ge&  (1-\dfrac{\mathbb{V}[N_{\text{pos}}]}{(\underline{N}_{\text{pos}}-n)^2}) \text{CDF}\left( n (d^++d^-) - N_{\text{cont}} d^-)(t^+-t^-) \right) + \dfrac{\mathbb{V}[N_{\text{pos}}]}{(\underline{N}_{\text{pos}}-n)^2} \text{CDF}\left( - N_{\text{cont}} d^-(t^+-t^-) \right) - \text{CDF}\left( 0 \right) \\
    :=& \tau(n)
\end{align}

By observing the monotonicity, it's obvious that the sufficient condition of $\alpha_{\text{rag}} < \alpha$ is $\hat{R}_{\text{rag}} < \hat{R}$. Therefore, we have the following from Hoeffding's inequality:
\begin{align}
    \sP\left[ \alpha_{\text{rag}} \le \alpha \right] &\ge \sP\left[ \hat{R}_{\text{rag}} \le \hat{R} \right] \\
    &\ge \max_n 1 - \exp\left\{ -2N_{\text{cal}}\tau(n)^2 \right\} - \dfrac{N_{\text{cont}}}{4(\underline{N}_{\text{pos}}-n)^2}
\end{align}
as long as $\tau(n)>0$.

Let $n=\dfrac{d^+ + 9d^-}{10(d^+ + d^-)}N_{\text{cont}}$. We finally have:
\begin{equation}
\begin{aligned}
    & \sP\left[ \alpha_{\text{rag}} < \alpha \right] \ge  1 - \exp\left\{ -2N_{\text{cal}} \left(\text{CDF}\left(\dfrac{(d^+-d^-) (t^+-t^-)}{10}N_{\text{cont}} \right) - \text{CDF}(0) \right)^2 \right\} \\ & - \dfrac{2025}{N_{\text{cont}}}  \left(\dfrac{d^+ }{d^+ + d^-}- \sum_{c=1}^C r_c^{\text{(cal)}} \left(N_{\text{ext}} - N_{\text{ext}} r_c^{\text{(ext)}} + {\sqrt{2\ln{10}}} \right)  \left(\ln \dfrac{\exp\left\{ -L_\tau \right\}}{1 - \exp\left\{ -L_\tau \right\}} \right)^{ -2N_{\text{ext}}r_c^{\text{(ext)}} +2 {\sqrt{2\ln{10}}} }   \right)^{-2}
\end{aligned}
\end{equation}
